# Supplementary material for: ComAct: Reframing Professional Software Manipulation via COM-as-Action Paradigm
Source: arXiv:2606.13239 source file (2026-06-30)
Supplement: Supplementary file 1 [file 10_appendix.tex]

\section{Appendix}
\begin{table*}[t]
  \centering
  \small
  \setlength{\tabcolsep}{8pt} % 调整列间距以填满页面
  \begin{tabular}{@{}lllr@{}}
    \toprule
    \textbf{Complexity} & \textbf{Task Category} & \textbf{Software} & \textbf{\# Samples} \\
    \midrule
    \multirow{3}{*}{\shortstack[l]{\textbf{Single-Task}\\($N=400$)}}
    & 3D Modeling & SolidWorks, Inventor & 200  \\
    & Assembly & Inventor & 100  \\
    & 2D Draft / Sketch & AutoCAD & 100  \\
    \midrule
    \multirow{4}{*}{\shortstack[l]{\textbf{Multi-Task}\\($N=600$)}}
    & 3D Modeling + Edit & SolidWorks, Inventor & 200  \\
    & 3D Modeling + Drawing & SolidWorks, Inventor & 100  \\
    & 3D Modeling + Mass Prop. & SolidWorks, Inventor & 200  \\
    & Assembly + Interference & Inventor & 100  \\
    \midrule
    \textbf{Total} & \textbf{All 7 Categories} & \textbf{SW, Inv, ACAD} & \textbf{1,000} \\
    \bottomrule
  \end{tabular}
  \caption{Overall statistics of \textbf{ComCADBench}.}
  \label{tab:comcadbench_statistics}
\end{table*}
